# Supplementary material for: Stochastic Games with Disjunctions of Multiple Objectives (Technical Report)
Source: arXiv:2108.04604 source file (2021-09-06)
Supplement: Supplementary file 1 [file 3b_SI.tex]

We propose a strategy iteration (SI) algorithm that computes the Pareto sets $\val(\game, \query)$ for a given DQ $\query$ in the standard semantics or $\upval(\game, \query)$ for a CQ $\query$ in the alternative ``will-know'' semantics.
%In order to use SI, we first have to ensure that the set of possible strategies to be finite.
%A natural way to do so is to construct the goal unfolding $\gunfold$, taking the product of the potential memory and the state space. In $\gunfold$, memoryless deterministic strategies suffice, and there are only finitely many of them.
%\todo{Define gunfold here or in prelims, prove that MD suffices (from strat compl?)}

SI typically works by iteratively fixing a strategy of one player, solving the induced MDP of the opponent and then improving the strategy locally according to the values in the induced MDP. 
In a single dimension, there is a total order on strategies, and thus this improvement eventually finds an optimal strategy $\straa^\ast$~\cite{HK66}. Then the value can be computed as the solution of the MDP $\G^{\straa^\ast}$.

For multi-objective queries, there is no total order on strategies, since they can be incomparable.
For example, consider the SG in  Figure~\ref{fig:introExample}. Note that the targets are absorbing, so the unfolding is trivial.
When fixing the strategy of $s_1$ to go to $T_1$, the Pareto set in $s_0$ is $\dwc(\nicefrac{1}{2},1)$, because anything with required probability of $T_1$ less than or equal to $\nicefrac{1}{2}$ is achievable, but \Achiever\ cannot rely on anything from state $s_2$. 
Dually, if $s_1$ plays the strategy of going to $T_2$, the Pareto frontier in $s_0$ is $\dwc(1,\nicefrac{1}{2})$.
Thus, the strategies are incomparable, as neither Pareto set is a subset of the other, i.e.\ no strategy is point-wise worse.
To get the full Pareto set in $s_0$, we have to take the union of the Pareto sets that result from all optimal strategies.

Thus, an SI algorithm cannot only rely on iteratively improving a \emph{single} strategy, but has to consider multiple improvements.
However, it can at least avoid using strategies that are strictly worse, similar to the improvement for our value iteration algorithm.
After fixing a strategy $\straa$ and solving the induced MDP $\G^{\straa}$ (e.g. using methods from~\cite{EKVY08}), for every state $s$ we obtain an estimate of the set of achievable points $\val(\game_s^{\straa}, \query)$ (where the $s$ in the index indicates that we consider $s$ as the initial state for the query).
We can then define the set of useful choices in a state $s$ as
\[
%\mathsf{uc}(s, \game^{^\straa(s)},\query) \eqdef 
\{t \in \choices(s) \mid \neg \exists t' \in \choices(s): \val(\game_t^{\straa}, \query) \subsetneq \val(\game_{t'}^{\straa}, \query)\}
\]
A choice is not useful if the achievable points from its successor are a strict subset of some other choice.
The strategy improvement step of our SI-style algorithm computes the set of all strategies that use useful choices (according to the achievable points in the current MDP) for all states. 
Denoting the useful choices of a state $s$ under a strategy $\straa$ as  $\mathsf{uc}(s,\straa)$, the improved or incomparable strategies are the set
\[\{\text{MD-strategy}~\straa' \mid \forall s\in \statesAll: \straa'(s) \in \mathsf{uc}(s,\straa) \}\]
In the end, the achievable points can be computed as the union over all considered strategies. We refer to Appendix~\ref{app:SI} for the pseudocode and correctness proof of our SI-style algorithm.

\begin{lemma}\label{lem:si-style}
	The SI-style algorithm terminates and returns the set of achievable vectors.
\end{lemma}
