# Supplementary material for: Stochastic Games with Disjunctions of Multiple Objectives (Technical Report)
Source: arXiv:2108.04604 source file (2021-09-06)
Supplement: Supplementary file 2 [file appendix_prelims.tex]

\subparagraph{Induced MDP and Markov chain}

\todo{obsolete?}\textcolor{orange}{We have it, so we can keep it. We use it implicitly; maybe refer to it somewhere after Definition 1?}
Given an SG $\game = (\Smax,\Smin,\Sprob,\sinit,P,\choices)$ and a strategy $\maxstrat$ of \Achiever\ in the general form $\maxstrat \colon S^*\Smax \to S$ (i.e.\ \emph{not} in terms of a memory automaton), we formally define the induced MDP $\game^\maxstrat$ as follows: Let $S = \Smax \cup \Smin \cup \Sprob$. $\game^\maxstrat$ is the countably infinite SG $(\Smax',\Smin',\Sprob',\sinit,P',\choices')$ where
\begin{itemize}
    \item $\Smax' \eqdef \emptyset$
    \item $\Smin' \eqdef S^* \Smin$
    \item $\Sprob' \eqdef S^* (\Sprob \cup \Smax)$
    \item For all $\path \in S^*$, $P'(\path s) \eqdef \begin{cases}
        \sigma(\path s) & \text{ if } s \in \Smax,\\
        P(s) & \text{ if } s \in \Sprob,
    \end{cases}$
    \item $\choices(\path s) \eqdef \{\path s t \mid t \in \choices(s) \}$ for all  $\path s \in \Smin'$.
\end{itemize}
The definition of $\game^\minstrat$ is completely analogous for a strategy $\minstrat$ of \Spoiler.
